# Supplementary material for: Telemanipulation with Chopsticks: Analyzing Human Factors in User Demonstrations
Source: arXiv:2008.00101 source file (2020-07-31)
Supplement: Supplementary file 1 [file study.tex]

\subsection{Study}

\begin{figure}[!htbp]
  \includegraphics[width=\linewidth]{figs/5.0.success_rate_on_teleop.png}
  \caption{Success rate for all subjects using teleoperation. Note that there is one subject that is outlier, so we remove all of its data in the paper.}
  \label{fig:outlier1}
\end{figure}

\begin{figure}[!htbp]
  \includegraphics[width=\linewidth]{figs/5.0.success_rate_all_subjects.png}
  \caption{Success rate for all subjects using all methods. Note that there is one subject that is outlier, so we remove all of its data in the paper.}
  \label{fig:outlier2}
\end{figure}
